# Supplementary material for: Structurally balanced growing network as randomized P\'olya urn process
Source: arXiv:2510.24659 ancillary file (2025-11-06)
Supplement: Supplementary file 1 [file supp.pdf]

# Supplemental Material for
# Structurally balanced growing network as randomized Pólya urn process

Krishnadas Mohandas,[1,*] Piotr J. Górski,[1,*] Krzysztof Suchecki,[1]
Georges Andres,[2] Giacomo Vaccario,[2] and Janusz A. Hołyst[1]

[1] *Faculty of Physics, Warsaw University of Technology, Koszykowa 75, PL 00-662 Warsaw, Poland*

[2] *Chair of System Design, ETH Zürich*

# Abstract

In this Supplemental Material, we present additional justifications for the analysis presented in the main text of the paper. This document contains eight supplemental figures, showing additional numerical results and supplemental text. The text describes the statistical characteristics of the clique size distribution, the theoretical formula of variance, and the applicability of the bimodality criterion in our growing network model.



* Authors contributed equally

# I. CONSTRUCTING BIMODAL DISTRIBUTION FROM UNIMODAL DISTRIBUTION

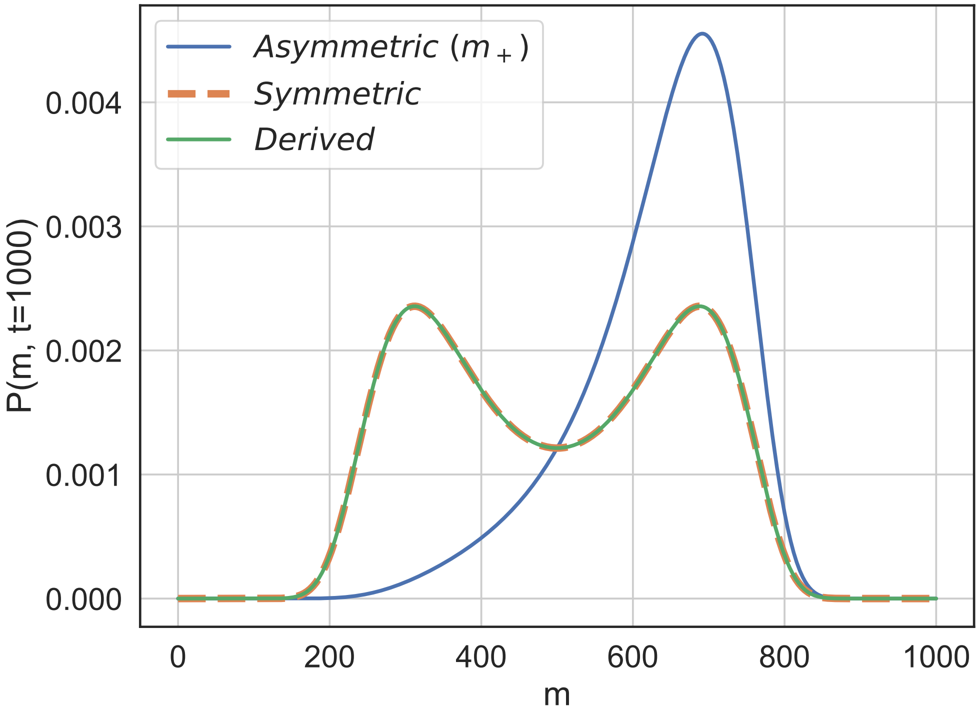


FIG. S1. A bimodal distribution can be formed by adding the individual distributions of both cliques through a reflection-based transformation. At time $t$, the distribution of one clique (blue line) is reflected about the midpoint $t/2$ to represent the distribution of the opposing clique (see Fig. 3 in the main text). The two are then averaged, scaling the sum by a factor of $\frac{1}{2}$ to preserve normalization, resulting in a bimodal distribution (green line) with two distinct peaks. For comparison, the dashed orange line shows the exact distribution obtained under the symmetric initial condition, demonstrating the equivalence of both construction methods.

# II. STATISTICAL CHARACTERISTICS

## A. Quantifying asymmetry using skewness

Skewness quantifies the asymmetry of a probability distribution around its mean [1], e.g., for the larger clique $m_+$, it is defined as

$$\alpha_3 = \mathbb{E}\left[\left(\frac{X - \langle m_+ \rangle}{\sigma_+}\right)^3\right], \tag{S1}$$

where $\sigma_+$ denotes the standard deviation of the unimodal distribution $P(m_+, t)$. A large absolute value of $\alpha_3$ indicates that the mean sizes of initially small and large cliques differ significantly. The skewness of the smaller clique is simply $-\alpha_3$.

As shown in the Fig. S2, $\alpha_3$ is increasingly negative with the increase of bias. It becomes visibly nonzero for $p \approx 0.7$, yet $\alpha_3$ is never exactly 0, but it is a monotonously decreasing function of $p$.

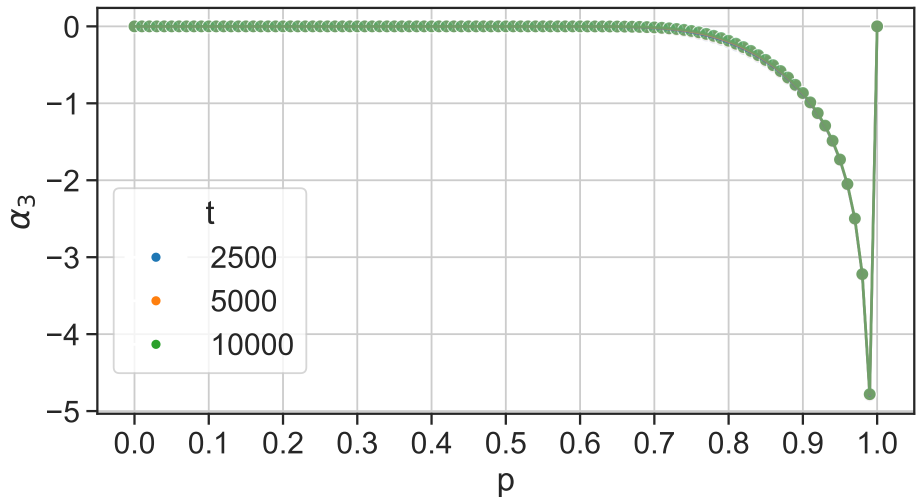


FIG. S2. Distribution asymmetry is a signature of the high $p$ regime. These trends are approximately independent of time. The plot shows the skewness $\alpha_3$, which decreases monotonically with $p$ and becomes noticeably nonzero only above $p \approx 0.75$. The results are obtained from the master equation using asymmetric initial conditions, ensuring exact values.

### B. Quantifying bimodality using excess kurtosis

The growth process can be characterized by time-dependent unimodal or bimodal distributions, each displaying distinct modal behavior. This is due to the concentration of probability mass around two distinct modes, rather than a single central peak [2]. This tends to "flatten" the overall shape compared to a normal distribution of similar variance. The modality of this distribution can be partially characterized by the excess kurtosis ($\alpha_4$) [3, 4] defined as

$$\alpha_4 = \mathbb{E}\left[\left(\frac{X - \langle m \rangle}{\sigma_\pm}\right)^4\right] - 3. \tag{S2}$$

Let us note that $\langle m \rangle$, the first moment of the combined distribution $P(m_{\pm}, t)$, is equal to $t/2$, while $\sigma_{\pm}$ denotes its standard deviation. A high value of excess kurtosis indicates a clear separation of peaks, highlighting a significant difference in sizes between the two cliques.

While some bimodal distributions exhibit negative excess kurtosis (often due to a flattened central region or dip), the specific dynamics governed by the parameter $p$ in our model leads to increasing absolute values of $\alpha_4$ as the bimodal structure develops [2, 4]. The observed bimodality emerges for sufficiently large values of $p$. Otherwise, the distribution remains unimodal and, on average, neither group dominates. Although negative kurtosis does not imply bimodality, it may indicate the existence of bimodality given the distribution is symmetric in a strict sense with only two local maxima [5]

Fig. S3 illustrates the calculated excess kurtosis $\alpha_4$ across a range of values for the parameter $p$ under both asymmetric and symmetric initial conditions. For asymmetric initial conditions, $\alpha_4$ approaches zero for anti-bias and low bias values of $p$, similar to symmetric initial conditions, but becomes positive for large $p$. Conversely, under the symmetric initial condition, $\alpha_4$ is negative in the high-bias regime, which is typically indicative of bimodal behavior [3]. However, a negative excess kurtosis alone is not sufficient to confirm bimodality.

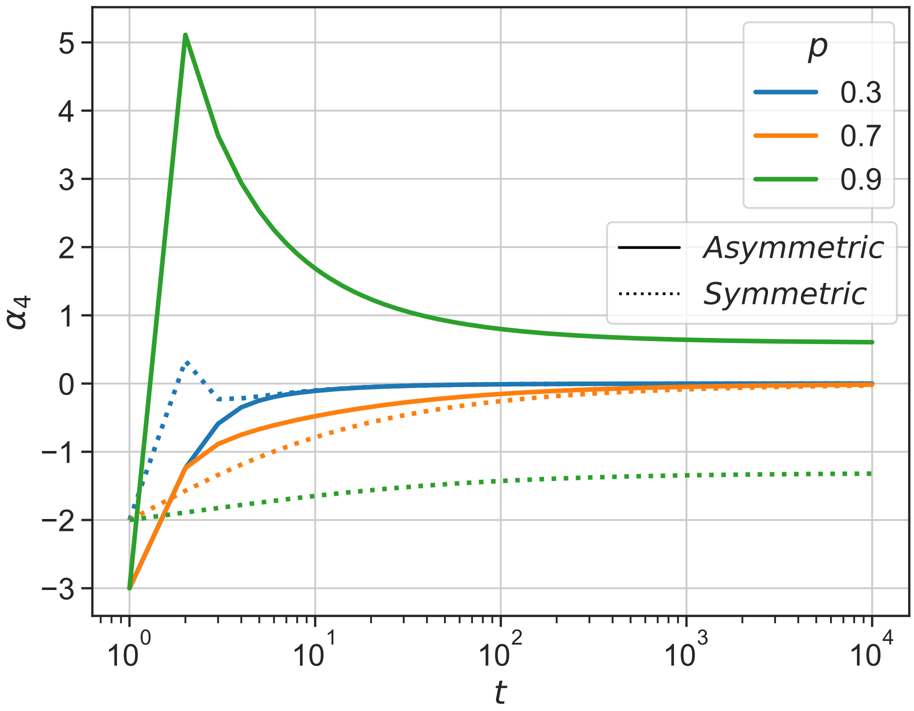


FIG. S3. Convergence of excess kurtosis $\alpha_4$ over time, with rates dependent on the attachment bias $p$ and initial conditions. The time evolution of excess kurtosis obtained from the distribution is shown for both asymmetric (solid) and symmetric (dotted) initial conditions. The measure $\alpha_4$ also converges to a limiting value, which can be zero, positive, or negative, determined by the attachment bias and initial conditions. For symmetric initial conditions, a negative $\alpha_4$ may correspond to the observed bimodal distribution.

### C. Mode of the distribution

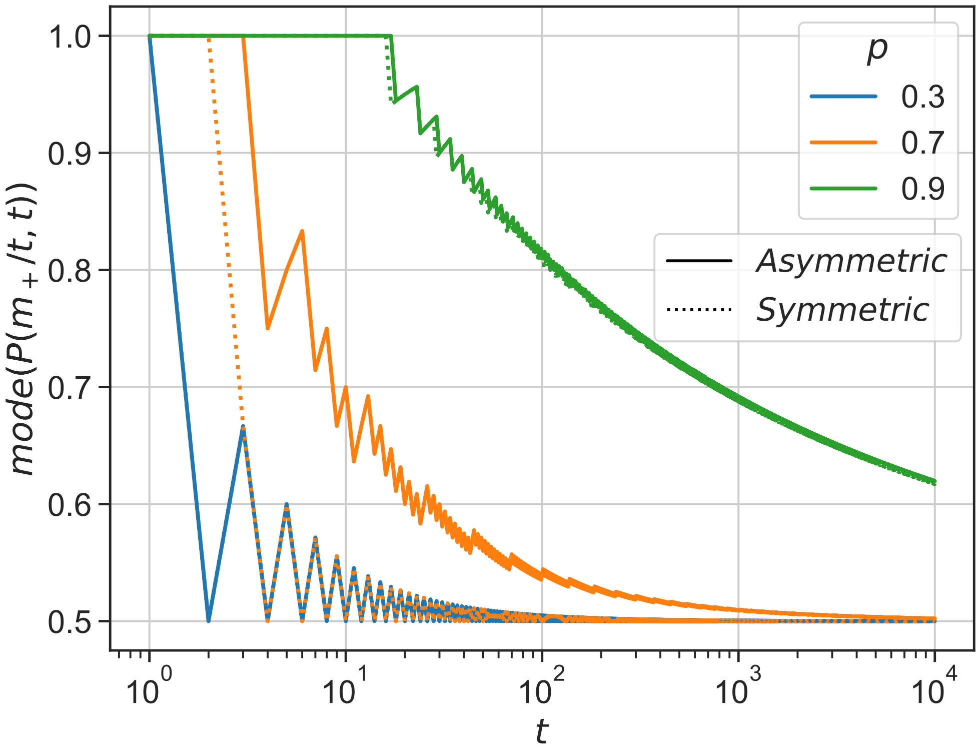


FIG. S4. Modes of the normalized distribution converge in time to 0.5, with the convergence rate dependent on the attachment bias $p < 1$ and initial conditions. For small or large values of $p$, the observed modes in both cases coincide. At shorter timescales, bimodal modes diverge from the original distribution's peaks but evolve toward 0.5 over longer periods, independently of $p$. However, for intermediate values of $p > 0.5$, the distributions in the two cases evolve differently, and the maxima diverge at shorter timescales. In all cases, the modes asymptotically converge to 0.5. The time evolution of normalized modes of larger clique size is shown for both asymmetric (solid) and symmetric (dotted) initial conditions. The observed "zig-zag" pattern is the consequence of the system's discrete nature.

### D. Mean under different initial clique size

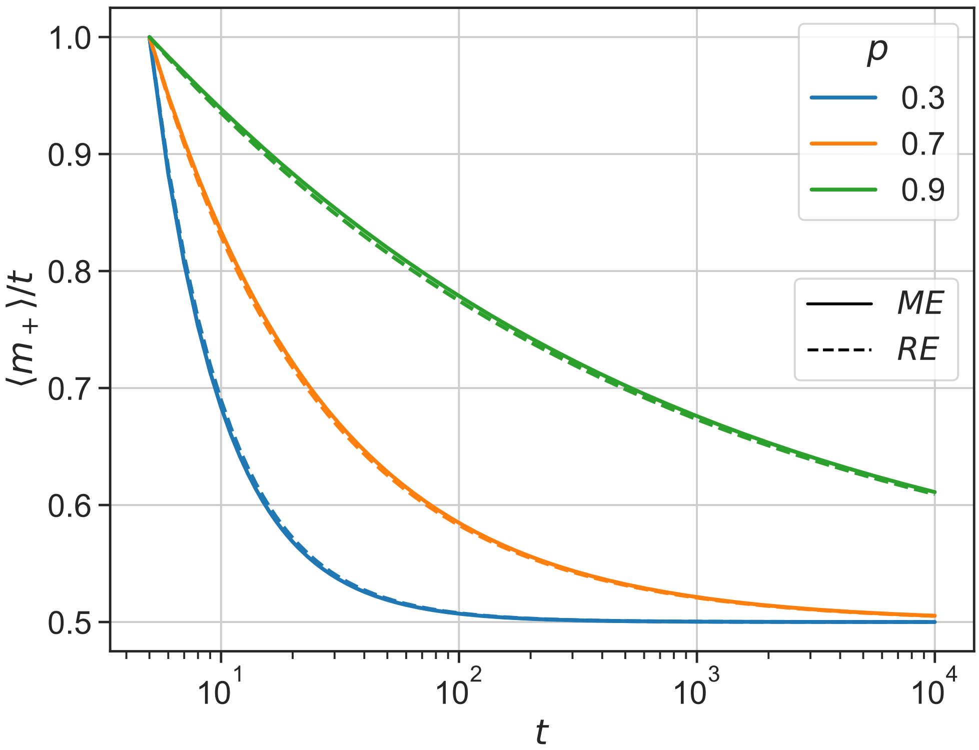


FIG. S5. The rate equation (RE) closely matches results derived from the master equation (ME), also when initially, the system consists of five nodes in a single clique. This shows that the rate equation is general for any initial conditions. The plot shows the time evolution of the normalized means for three different attachment bias $p$ values.

## III. EQUIVALENCE OF GROWING NETWORK MODEL AND PÓLYA-LIKE PROCESS

In our derivation of equations related to the Pólya process and its equivalence to our growing model, we broadly used the results presented in [6]. Janson [6] introduced a matrix $A$ whose elements $a_{ij}$ describe how many balls of color $j$ are added when a ball of color $i$ is drawn. In general, the elements $a_{ij}$ can be random variables drawn from a given distribution. When only two colors are considered, the matrix $A$ takes the form:

$$A = \begin{pmatrix} a_{11} & a_{12} \\ a_{21} & a_{22} \end{pmatrix}.$$

The eigenvalues of the matrix $A$ are key to understanding the behavior of the system. The largest eigenvalue $\lambda_1$ is real and positive. For Markov branching processes, such as the Pólya process, the long-term behavior depends on whether the second largest eigenvalue $\lambda_2$ is such that $\mathrm{Re}(\lambda_2) > \lambda_1/2$. For such systems, the mean grows like $t^{\lambda_1}$, while the variance grows like $t^{2\lambda_2}$.

The growing network model considered in our study is equivalent to a Pólya process with two colors, where the probability of adding a ball of a different color (than the one drawn) is the same for both colors. In that case, the matrix $A$ becomes:

$$A = \begin{pmatrix} p & 1-p \\ 1-p & p \end{pmatrix},$$

where $p$ corresponds to the bias parameter introduced in the main text.

This case corresponds to the "Randomized play-the-winner" process (Example 7.3 in [6]), originally introduced in [7]. The eigenvalues of $A$ in this setting are $\lambda_1 = 1$ and $\lambda_2 = 2p - 1$. Applying the condition $\lambda_2 > \lambda_1/2$ yields a threshold at $p = 0.75$. For this example, using Theorems 3.22 and 3.23 from [6], one can derive the asymptotic distributions for $p \leq 0.75$ with equal expected sizes of both cliques and variances given below.

For $p > 0.75$, the process lacks a closed-form limit distribution. In this case, we applied Theorem 3.24 using the setting described in Example 3.27 of [6], which considers deterministic numbers of balls added (i.e., all elements of matrix $A$ are deterministic).

This allows the derivation of the limiting distribution and expected values presented in the main text.

$$t^{-(2p-1)} \left( m_{\pm} - \frac{t}{2} \right) \xrightarrow{\text{a.s.}} \pm \frac{1}{2} \hat{Z}, \tag{S3}$$

where $\hat{Z}$ is a distribution. When starting with a single ball of given color, the moments of $\hat{Z}$ can be computed by Theorem 3.26 of [6] as

$$\mathbb{E}\hat{Z}^k = \frac{1}{\Gamma\left(1 + k(2p-1)\right)} \mathbb{E}Z^k, \tag{S4}$$

where, following Example 3.13 of [6], $\mathbb{E}Z = 1$ and variance $V(Z) = \dfrac{(2p-1)^2}{4p-3}$. This allows calculation of $\mathbb{E}Z^2$ and, further $\mathbb{E}\hat{Z}$, $\mathbb{E}\hat{Z}^2$ and finally $Var(\hat{Z})$.

### A. Variance analysis

Summing up the previous text, the derived formulae for the expected variance for different values of attachment bias $p$ are as follows:

$$\mathrm{V}_{p,t} = \begin{cases} \dfrac{t}{4(3-4p)}, & \text{for } p < 0.75, \\ \dfrac{t\log t}{4}, & \text{for } p = 0.75, \\ \dfrac{t^{2(2p-1)}}{2}\left(\dfrac{1}{\Gamma(4p-1)}\cdot\dfrac{4p^2-2}{4p-3} - \left(\dfrac{1}{\Gamma(2p)}\right)^2\right), & \text{for } p > 0.75. \end{cases} \tag{S5}$$

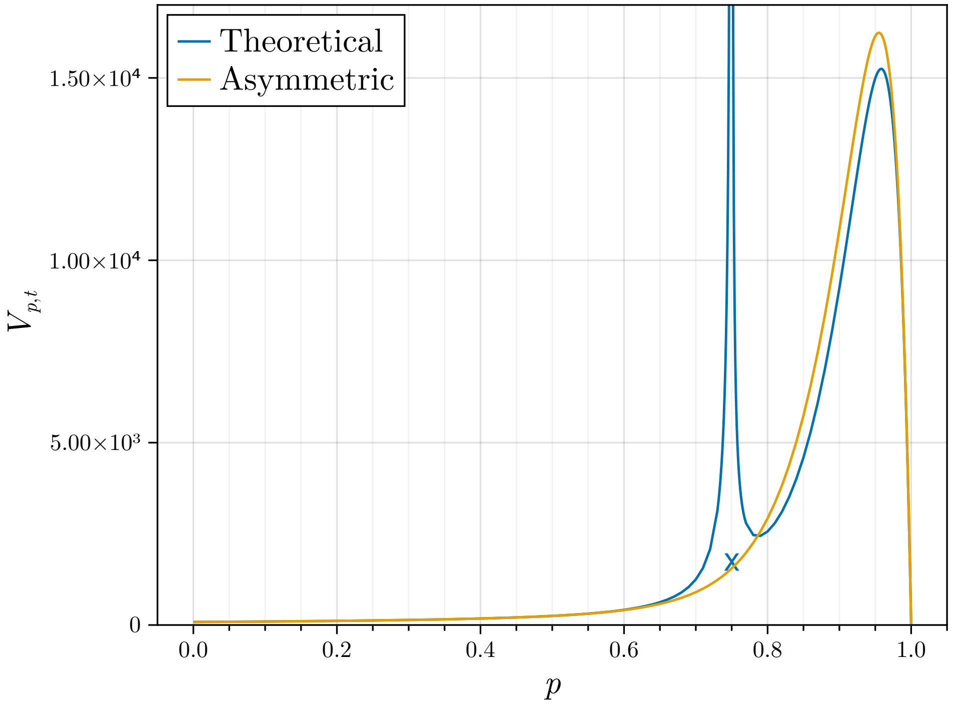


FIG. S6. Variance of the clique size under asymmetric initial conditions with a single starting node for different values of $p$. The theoretical variance (blue line) calculated using Pólya process analysis (Eq. S5) diverges at $p \to 0.75$, which is inconsistent with the true variance (orange line) obtained using the master equation. The plot shows the variance after $t = 1000$ steps.

Fig. S6 compares the theoretical variance with the exact values obtained from the master equation. For $p \lesssim 0.65$, the theoretical predictions are equivalent to the true variance. However, the analytical expressions for the two regimes, $p < 0.75$ and $p > 0.75$, diverge at

the critical point $p = 0.75$. As a result, the discrepancy between theory and exact values increases as $p$ approaches this threshold from either side. Interestingly, the expression for $p = 0.75$ provides variance estimates that differ only slightly from the exact values, much like the deviations seen for $p \gtrsim 0.8$.

The discrepancy between analytics and simulation results arises from the breakdown of assumptions made in the theoretical approximations. For $p < 0.75$, the analytical expression relies on a central limit theorem-type behavior, assuming that fluctuations scale linearly with time, i.e., as $t$. For $p > 0.75$, a different scaling is assumed, with fluctuations growing superlinearly as $t^{2(2p-1)}$. Both assumptions hold well away from the critical point. However, near the critical point $p = 0.75$, they break down: the transition between the linear and superlinear scaling is not abrupt but smooth, and neither scaling form captures the correct fluctuation behavior precisely. As a result, the variance predicted analytically diverges at $p = 0.75$, while the true (numerical) variance remains finite and follows a logarithmic correction.

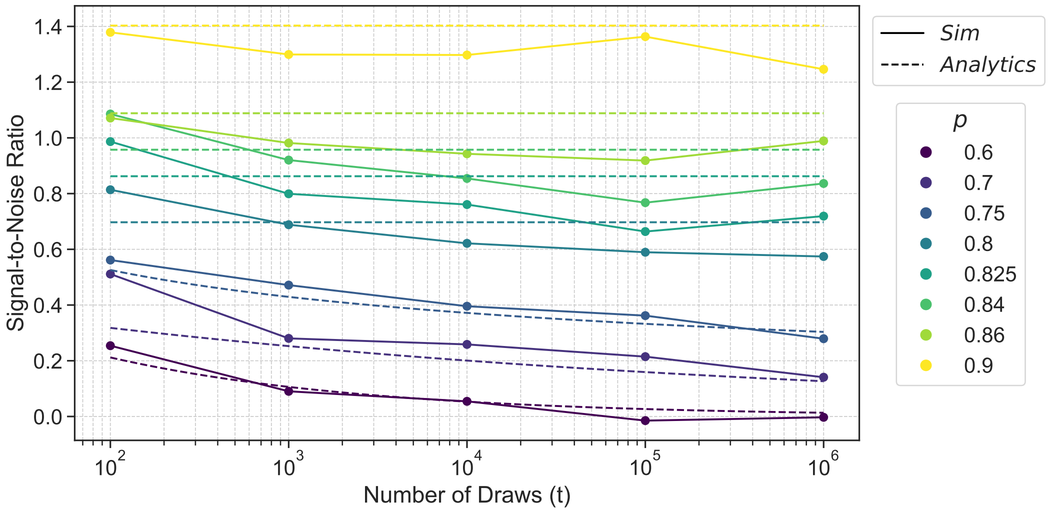


FIG. S7. SNR as a way to estimate the relationship between the mean faction sizes and fluctuations. In the low bias regime $p < 0.75$, it becomes increasingly difficult to detect any difference in the faction sizes as the system grows. At $p = 0.75$, the SNR decreases, but this decrease is very slow. In the high Bias Regime ($p > 0.75$), SNR is a constant. This constancy indicates that in this regime, the difference in faction sizes is more stable and detectable

## IV. MEASURING CHARACTERISTIC BIAS

### A. Asymptotic characteristic bias

The second derivative of the distribution, evaluated at $m = t/2$, i.e., $\frac{d^2P(m,t)}{dm^2}|_{m=t/2}$, provides a straightforward criterion to distinguish between unimodal and bimodal distributions. For each time $t$, the characteristic bias $p_t^{ch}$ is estimated by linearly interpolating between the two points immediately before and after the crossing $\frac{d^2P(m,t)}{dm^2}|_{m=t/2} = 0$. The resulting values of $p_t^{ch}$ for various $t$ are shown in Fig. S8a.

To determine the asymptotic characteristic bias $p_\infty^{ch}$, we analyzed the convergence of $p_t^{ch}$ by fitting a power-law relation

$$\log|p_t^{ch} - p_\infty^{ch}| \sim \log t, \tag{S6}$$

where $p_\infty^{ch}$ is chosen to maximize the coefficient of determination $R^2$ of the linear fit. The quality of the fit and the resulting $p_\infty^{ch}$ are shown in Fig. S8b.

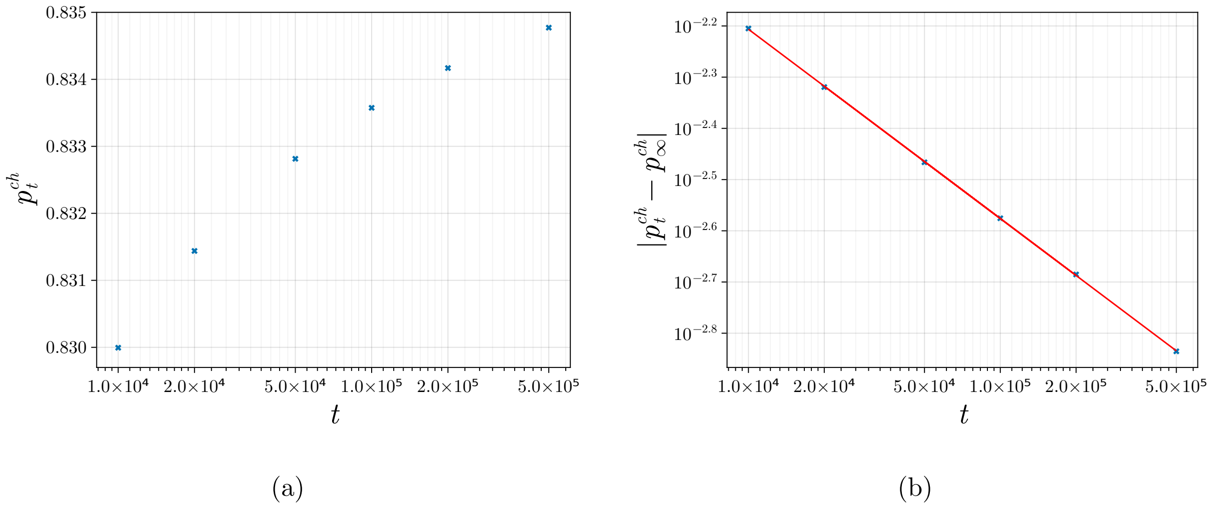


FIG. S8. Convergence of characteristic bias $p^{ch}$ over time. Panel (a) shows that the characteristic bias $p_t^{ch}$ increases monotonically. Panel (b) depicts the relation between the absolute difference $|p_t^{ch} - p_\infty^{ch}|$ and time $t$ on a double logarithmic scale. The fitted line follows a power-law scaling, $\log|p_t^{ch} - p_\infty^{ch}| \sim \log t$. The asymptotic value $p_\infty^{ch}$ was determined by maximizing the coefficient of determination $R^2$ of the fit. For the obtained fit, $R^2 > 0.9999$. The results are shown when starting from a single-node symmetric initial condition.

### B. Characteristic bias based on observability criterion

A criterion for assessing bimodality (Eq. (9)) indicates a higher value of characteristic $p^{ch}$. However, it is essential to note that this criterion is based on an approximation that is valid only for Gaussian distributions. Therefore, the value obtained through the numerical analysis will be regarded as the more accurate one. The key insight lies in the sign of

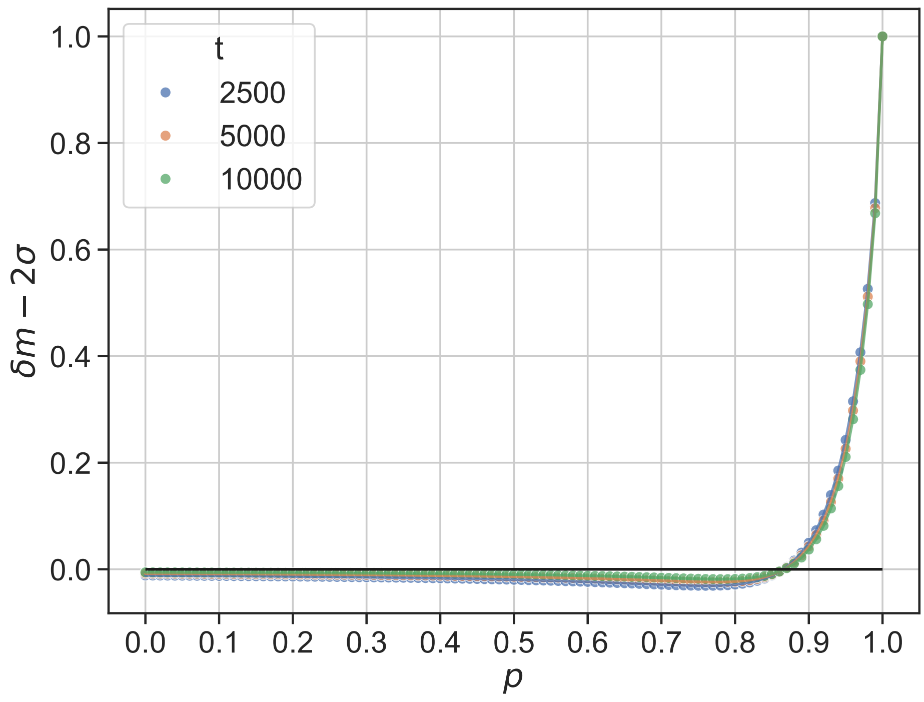


FIG. S9. A criterion based on Gaussian approximation (9) predicts the emergence of bimodality when the separation between the normalized peaks $\delta m = (m_+ - m_-)/t$ exceeds twice the standard deviation $\sigma$ of the normalized distribution under the asymmetric initial condition. For values of attachment bias $p > 0.86$, this condition is met, suggesting the potential for a bimodal distribution if symmetric initial conditions are applied. When the difference is negative, the peaks are expected to merge, resulting in a unimodal distribution.

the quantity $\delta m - 2\sigma$, where $\delta m$ is the normalized gap between larger and smaller clique ($\delta m = \Delta m/t$), and $\sigma$ is the standard deviation of the normalized distribution (Fig. S9). When $p \gtrsim 0.86$, this quantity becomes positive, indicating that the two peaks are sufficiently separated to prevent overlap, and a bimodal distribution emerges. For $p \lesssim 0.86$, the quantity is negative, implying that fluctuations obscure any separation between maxima, resulting in

a unimodal distribution. The final result appears to be inconsistent with numerical findings from Sec. VI, where the characteristic value of $p^{ch} \approx 0.836$ was identified. It is important to note that the criterion itself is an approximation, valid only for Gaussian distributions. Nevertheless, the criterion proves effective in practice.

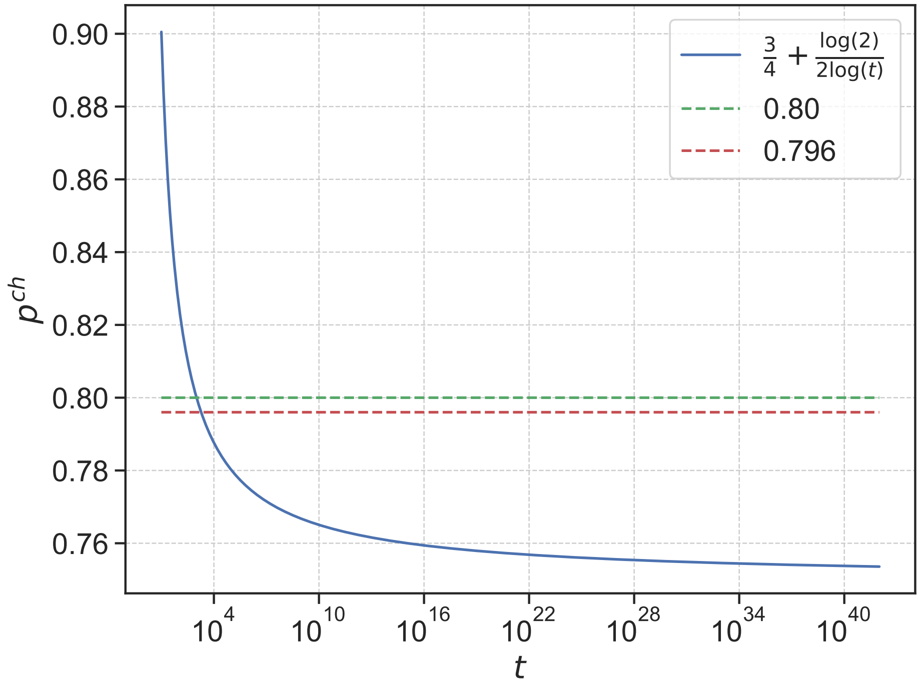


FIG. S10. Analytical threshold for bimodality derived by considering the growth process as an equivalent unbiased random walk. At $t \to \infty$, the threshold tends to 0.75. The characteristic thresholds at $t = 1000$ and $t = 2000$ result in $p \gtrsim 0.801$ and $p \gtrsim 0.796$ respectively, which align with the results in 4, where bimodality emerges only for $p = 0.9$.

---


[1] R. B. D'Agostino, *Goodness-of-fit-techniques*, Vol. 68 (CRC press, 1986).

[2] J. B. Freeman and R. Dale, Behav Res Methods **45**, 83 (2013).

[3] R. B. D. and, Am. Stat. **24**, 19 (1970).

[4] K. P. Balanda and H. L. M. and, Am. Stat. **42**, 111 (1988).

[5] T. Wyszomirski, J. Theor. Biol. **158**, 109 (1992).

[6] S. Janson, Stochastic Processes and their Applications **110**, 177 (2004).

[7] L. Wei and S. Durham, J. Am. Stat. Assoc. **73**, 840 (1978).
